# Supplementary material for: Early-Bird Diffusion: Investigating and Leveraging Timestep-Aware Early-Bird Tickets in Diffusion Models for Efficient Training
Source: arXiv:2504.09606 source file (2025-04-13)
Supplement: Supplementary file 3 [file sm_ddpm_church_eb.tex]

\begin{table}
\centering
\caption{EB Tickets with 50\% pruning rate on LSUN Church with 256 $\times$ 256 resolution using the DDPM \cite{ho2020denoising}. The best FID score is highlighted in \textbf{bold}. The ``Early Bird'' column denotes the pseudo-epoch of 1000 steps in which the subnetwork is sampled at.}
\vspace{-0.5em}
\scriptsize 
\setlength{\tabcolsep}{4pt} 
 
\resizebox{\linewidth}{!}{ 
\begin{tabular}{@{}lcccccc@{}}
\toprule
\multirow{2}[2]{*}{\tabincell{l}{\textbf{Pruning}\\\textbf{Metric}}} & \multicolumn{5}{c}{\textbf{DDPM @ LSUN Church (256$\times$256)}}
\\
\cmidrule(lr){2-6}
 & \textbf{\# Params} $\downarrow$ & \textbf{MACs} $\downarrow$ & \textbf{FID} $\downarrow$ & \textbf{Early Bird} & \textbf{Iters} \\
\midrule
\multirow{2}{*}{\shortstack[l]{Magnitude \\ Taylor}} 
& \multirow{2}{*}{19.7M} & \multirow{2}{*}{6.0G} & 37.6 & 14 & 800K\\
 & & & \tobeadded{???} & \tobeadded{???} & 800K\\
\bottomrule
\vspace{-2.5em}
\end{tabular}
}
\label{tab:ddpm_lsun_church}
\end{table}
