# Supplementary material for: Early-Bird Diffusion: Investigating and Leveraging Timestep-Aware Early-Bird Tickets in Diffusion Models for Efficient Training
Source: arXiv:2504.09606 source file (2025-04-13)
Supplement: Supplementary file 4 [file sm_imagenet_taeb.tex]

\begin{table}[t]
    \centering
    \vspace{-1em}
    \caption{Results for \textbf{TA-EB} ImageNet-1K using the LDM \cite{rombach2021highresolution}. The number of iterations are recorded as the total number of iterations for the subnetwork with the longest training time.}
    \vspace{-0.5em}
    \resizebox{\columnwidth}{!}{%
    \begin{tabular}{lcccc}
    \toprule
    \multirow{2}{*}{\textbf{Pruning Metric}} & \multicolumn{4}{c}{\textbf{LDM @ ImageNet (256$\times$256)}} \\
    \cmidrule(lr){2-5}
    & \textbf{\#Params $\downarrow$} & \textbf{MACs $\downarrow$} & \textbf{FID $\downarrow$} & \textbf{Iters} \\
    \midrule
    Magnitude & 267.5M & 117.3G & 44.63 & 50K \\
    Taylor & 267.5M & 117.3G & \tobeadded{???} & 50K \\
    \bottomrule
    \end{tabular}
    }
    \label{tab:imagenet_ldm}
\end{table}
